# Supplementary material for: On the variance of radio interferometric calibration solutions: Quality-based Weighting Schemes
Source: arXiv:1711.00421 source file (2018-02-06)
Supplement: Supplementary file 1 [file appendix.tex]

\section{Mathematical Demonstrations}\label{app.maths}

\subsection{Expliciting $\matVV$}\label{app.sec.matvv}

\pg
We have defined $\matVV$ in Eq. \ref{eq.matvv.definition} as:
\begin{align}
\matVV             =& \Rmat{}^H \Rmat{} %\\
%                   =& (\sum_d s_d \Kmat{d} \Varmat \Kmat{d}^H)^H(\sum_d s_d \Kmat{d} ( \Varmat ) \Kmat{d}^H)\\
%                   =& (\sum_d s_d \Kmat{d}^H \Varmat^H \Kmat{d})(\sum_d s_d \Kmat{d} ( \Varmat ) \Kmat{d}^H)\\
%                   =& \Varmat^H \Varmat \sum_d \sum_{d'} s_ds_{d'}\Kmat{d}^H\Kmat{d} \Kmat{d'}\Kmat{d'}^H
%\matVV[\tnuIndeix,\tnuIndeix']  =& \Exp{(\Varmat\sum_d s_d \Kmat{d})^H(\Varmatprime\sum_d s_d \Kmat{d})} + \mathbf{{I}} \sigma^2\\
%                   =& \Exp{\Varmat^H\Varmatprime}\sum_{d,d'}s_ds_{d'}\Kmat{d}^H\Kmat{d'} + \mathbf{{I}} \sigma^2\\
%\Exp{\Varmat^2}    =& (\matVV - \mathbf{{I}} \sigma^2)\hadam (\sum_{d,d'}s_ds_{d'}\Kmat{d}^H\Kmat{d'})^{\hadam-1} 
\end{align}
For a given $[\cellindex,\cellindex']$ cell, $\matVV$ becomes:
\begin{align}
\matVV[\cellindex,\cellindex'] =& \sum_{\tnuIndeix\in\cellindex} (\sum_ds_d\Kmat{d,\tnuIndeix}\VarmatTau\Kmat{d,\tnuIndeix}^H)^H(\sum_{d}s_d\Kmat{d,\tnuIndeix'}\VarmatTauprime\Kmat{d,\tnuIndeix'}^H)\\
                               =& \sum_{\tnuIndeix\in\cellindex} (\sum_ds_d\Kmat{d,\tnuIndeix}\VarmatTau^H\Kmat{d,\tnuIndeix}^H)(\sum_{d}s_d\Kmat{d,\tnuIndeix'}\VarmatTauprime\Kmat{d,\tnuIndeix'}^H)\\
                               =& \sum_{\tnuIndeix\in\cellindex} \sum_{d,d'}s_ds_d'\Kmat{d,\tnuIndeix}\VarmatTau^H\Kmat{d,\tnuIndeix}^H\Kmat{d',\tnuIndeix'}\VarmatTauprime\Kmat{d',\tnuIndeix'}^H \label{eq.vector.varmatccprime}
                               %=& \sum_{\tnuIndeix\in\cellindex} (\sum_ds_d\Kmat{d,\tnuIndeix}\Kmat{d,\tnuIndeix}^H) \VarmatTau^H\VarmatTauprime (\sum_ds_d\Kmat{d,\tnuIndeix'}^H\Kmat{d,\tnuIndeix'})^H \\
                               %=& \sum_{\tnuIndeix\in \cellindex} \kappamat{\tnuIndeix} \VarmatTau^H \VarmatTauprime \kappamat{\tnuIndeix'}       \leftrightarrow \sum_{\tnuIndeix\in \cellindex} \VarmatTau^H \kappamat{\tnuIndeix} \kappamat{\tnuIndeix'} \VarmatTauprime
%                               =& \sum_{\tnuIndeix\in \cellindex}\VarmatTau^H \VarmatTauprime \sum_d \sum_{d'} s_ds_{d'}\kappamat{d,\tnuIndeix}\kappamat{d',\tnuIndeix'}^H
\end{align}
where we define:
\begin{align}
%\kappamat{\tnuIndeix} =& \sum_d\Kmat{d,\tnuIndeix}\Kmat{d,\tnuIndeix}^H\\
\tnuIndeix'           =& \tnuIndeix+\Delta \tnuIndeix
\end{align}
with $\Delta\tnuIndeix$ corresponding to the shift in time and frequency to go from one cell to the other. In other words, the cells must be the same size, and the residual visibilities must be projected from one cell onto the other - we have no cross terms in the sum over $\tnuIndeix,\tnuIndeix'$.

\pg
If the model is dominated by bright point sources, the cross-terms in the sum over $d$ in Eq. \ref{eq.vector.varmatccprime} will be negligible (cf. Eq. \ref{eq.dirfunc.def}). We then have
\begin{align}
 &\sum_{d,d'}s_ds_d'\Kmat{d,\tnuIndeix}\VarmatTau^H\Kmat{d,\tnuIndeix}^H\Kmat{d',\tnuIndeix'}\VarmatTauprime\Kmat{d',\tnuIndeix'}^H\\
=&\sum_d s_d^2  \Kmat{d,\tnuIndeix}\VarmatTau^H\Kmat{d,\tnuIndeix}^H\Kmat{d,\tnuIndeix'}\VarmatTauprime\Kmat{d,\tnuIndeix'}^H
\end{align}
and we are left with
\begin{align}
\matVV[\cellindex,\cellindex'] =& \sum_{\tnuIndeix\in\cellindex} \sum_{d}s_d^2\Kmat{d,\tnuIndeix}\VarmatTau^H\Kmat{d,\tnuIndeix}^H\Kmat{d,\tnuIndeix'}\VarmatTauprime\Kmat{d,\tnuIndeix'}^H % + \Order{dd'}
\end{align}

\pg
In the diagonal cells of $\matVV$, we have:
\begin{align}
\matVV[\cellindex,\cellindex] =& \sum_{\tnuIndeix\in\cellindex}( \sum_{d}s_d^2\Kmat{d,\tnuIndeix}\VarmatTau^H\underbrace{\Kmat{d,\tnuIndeix}^H\Kmat{d,\tnuIndeix}}_{=\I}\VarmatTauprime\Kmat{d,\tnuIndeix}^H + \I\sigma^2)\\
                              =& \sum_{\tnuIndeix\in\cellindex}(\sum_ds_d^2 \Kmat{d,\tnuIndeix} \VarmatTau^H\VarmatTau \Kmat{d,\tnuIndeix}^H + \I\sigma^2)\\
                              =& \sum_{\tnuIndeix\in\cellindex}(\sum_ds_d^2\VarmatTau^H\VarmatTau \hadam(\kvect{d,\tnuIndeix}\kvect{d,\tnuIndeix}^H) + \I\sigma^2)\\
                              %=& \sum_{\tnuIndeix\in\cellindex}(\sum_ds_d^2\VarmatTau^H\VarmatTau \hadam(\kvect{d,\tnuIndeix}\kvect{d,\tnuIndeix}^H) + \I\sigma^2)\\
         \kvect{d,\tnuIndeix} =& \diag{\Kmat{d,\tnuIndeix}}
\end{align}
